# Supplementary material for: Algorithmic Robust Forecast Aggregation
Source: arXiv:2401.17743 source file (2024-01-31)
Supplement: Supplementary file 1 [file appendix.tex]

\section{Second Order}
% \section{Additional material (should not be included)}
Here is an example showing 
\fang{some comments on ratio objective}
We show our problem has a \emph{downward scale-invariant property}.  Given an aggregator $f$ and an information structure $\theta$ with prior $\mu$, as defined in \cite{DBLP:journals/corr/abs-2111-03153} the value of aggregator $f$ is defined as $$v(f, \theta) := \E_\theta[\ell(\mu, w)]-\E_\theta[\ell(f(x), w)]$$
where $\mu$ is the constant function that outputs the prior, and ratio of value and regret are $$Ratio(f, \theta):=v(f,\theta)/v(opt_\theta, \theta), \text{ and }R(f, \theta) = v(opt_\theta, \theta)-v(f, \theta).$$  
\begin{proposition}
For any $0<\epsilon\le 1$, information structure $\theta$,  and aggregator $f$, there exists an information structure $\theta_\epsilon$ so that 
$$Ratio(f, \theta_\epsilon)\le Ratio(f, \theta)\text{ and }v(opt_{\theta_\epsilon}, \theta_\epsilon) = \epsilon v(opt_{\theta}, \theta).$$
\end{proposition}
Therefore, to maximize the (worst) minimum ratio, we only need to consider information structures with almost zero information value $v(opt_{\theta_\epsilon}, \theta_\epsilon)$.\fang{by a proper choice of $\epsilon$, we can also make $R(f, \theta_\epsilon)$ arbitrarily close to zero}\fang{This result goes beyond conditional independent information structures but needs a flexible signal space}
\begin{proofsketch}
    Given an arbitrary information structure $\theta$, consider a $\epsilon$-noise operator (also known as garbling) $\theta\to \theta_\epsilon$ which outputs a mixture of the original information with probability $\epsilon$ and an uninformative new signal otherwise.  Hence, $\theta_\epsilon$ satisfies the second condition
    \begin{align*}
        &v(opt_{\theta_\epsilon}, \theta_\epsilon)\\
        =& \E_{w\sim \mu}[\ell(\mu, w)]-\E_{\theta_\epsilon}[\ell(opt_{\theta_\epsilon}, w)]\tag{$\theta$ and $\theta_\epsilon$ has the same prior}\\
        =& \E_{w\sim \mu}[\ell(\mu, w)]-\left(\epsilon\E_{\theta}[\ell(opt_{\theta}, w)]+(1-\epsilon)\E_{w\sim \mu}[\ell(\mu, w)]\right)\tag{posterior of uninformative signals is prior}\\
        =& \epsilon\left(\E_{w\sim \mu}[\ell(\mu, w)]-\E_{\theta}[\ell(opt_{\theta}, w)]\right)\\
        =& \epsilon v(opt_{\theta}, \theta).
    \end{align*} 
    On the other hand, because for all $\mu'$ the expected quadratic loss satisfies $\E_{w\sim \mu}[\ell(\mu', w)]\ge \E_{w\sim \mu}[\ell(\mu, w)]$, we have
    \begin{align*}
        &v(f, \theta_\epsilon)\\
        =& \E_{w\sim \mu}[\ell(\mu, w)]-\E_{\theta_\epsilon}[\ell(f(x), w)]\\
        =& \E_{w\sim \mu}[\ell(\mu, w)]-\left(\epsilon \E_\theta[\ell(f(x), w)]+(1-\epsilon)\E_{w\sim \mu}[\ell(f(\mu, \mu), w)]\right)\tag{posteriors are $\mu$ given uninformative information}\\
        \le& \E_{w\sim \mu}[\ell(\mu, w)]-\left(\epsilon \E_\theta[\ell(f(x), w)]+(1-\epsilon)\E_{w\sim \mu}[\ell(\mu, w)]\right)\tag{$f(\mu, \mu)\to \mu$ can decrease loss}\\
        =& \epsilon\left(\E_{w\sim \mu}[\ell(\mu, w)]-\E_\theta[\ell(f(x), w)]\right)\\
        =& \epsilon v(f, \theta)
    \end{align*}
    Therefore, by the above inequalities, $Ratio(f, \theta_\epsilon)\le Ratio(f, \theta)$.
\end{proofsketch}

\subsection{TVD to EMD}
In this section, we show two results that can upper bound the EMD of predictions or higher order predictions distributions by the TVD of signals distributions.

\begin{proposition}\label{prop:tv2first}
    Given two information structures $\theta$ and $\theta'$ on $\Omega\times \mathcal{S}_1\times\mathcal{S}_2$, 
    $$d_{EM}(\Xdis{\theta},\Xdis{\theta'})\le 6d_{TV}(\Sigdis{\theta}, \Sigdis{\theta'})$$
    where $\Sigdis{\theta}$ is the random variable of the state and signals sampled from the information structure with $\theta$.
\end{proposition}
\begin{proof}[Proof of \Cref{prop:tv2first}]
Let $d_{TV}(\Sigdis{\theta},\Sigdis{\theta'}) = \delta$.  Our coupling is derived from the maximal coupling between information structures $\theta$ and $\theta'$ on the signal space.  Informally, we first sample the signals from the maximal coupling and map the signals to predictions.  Specifically, we sample ${\vs}$ with probability $\Pr_\theta[{\vs}]$ and output $\hat{\mathbf{X}} = (\Pr_\theta[W|{s_1}], \Pr_\theta[W|{s_2}])$.  Then, let $\hat{\mathbf{X}}' = (\Pr_{\theta'}[W|{s_1'}], \Pr_{\theta'}[W|{s_2'}])$ with probability $\min(1, \Pr_{\theta}[{\vs}]/\Pr_{\theta'}[{\vs}])$ and any other feasible value that satisfies the marginal distribution so that $\hat{\mathbf{X}} = \Xdis{\theta}$ and $\hat{\mathbf{X}}' = \Xdis{\theta'}$ in distribution.

Let $d_{TV}(\Sigdis{\theta}, \Sigdis{\theta'}) = \delta$.  First we define the matching event as  
    $$\mathcal{E}:=\{(\hat{\mathbf{X}}, \hat{\mathbf{X}}'): \exists \vs, \hat{\mathbf{X}} = \Pr_\theta[W|\vs], \hat{\mathbf{X}}' = \Pr_{\theta'}[W|\vs]\}.$$  Then the probability of not matching is 
    \begin{equation}\label{eq:tv2first1}
        1-\sum_{\vs}\Pr_\theta[\vs]\frac{\min(\Pr_\theta[\vs], \Pr_{\theta'}[\vs])}{\Pr_\theta[\vs]} = \frac{1}{2}\sum_{\vs}|\Pr_\theta[\vs]-\Pr_{\theta'}[\vs]| = d_{TV}(\mathbf{S}_\theta,\mathbf{S}_{\theta'})\le\delta
    \end{equation}
    The second equality is due to \Cref{def:tvd}.  By the duality form of EMD in~\Cref{eq:dual}, we have
    $$d_{EM}(\Xdis{\theta},\Xdis{\theta'})\le \E\left[\|\hat{\mathbf{X}}-\hat{\mathbf{X}}'\|_1\right] = \E\left[\|\hat{\mathbf{X}}-\hat{\mathbf{X}}'\|_1\mid \neg \mathcal{E}\right]\Pr[\neg \mathcal{E}]+\E\left[\|\hat{\mathbf{X}}-\hat{\mathbf{X}}'\|_1\mid \mathcal{E}\right]\Pr[\mathcal{E}].$$
    We bound these two terms separately. First, because the one norm of the difference between two distributions is always bounded by $2$, with \Cref{eq:tv2first1}
    $$\E\left[\|\hat{\mathbf{X}}-\hat{\mathbf{X}}'\|_1\mid \neg \mathcal{E}\right]\Pr[\neg \mathcal{E}]\le \max_{\vx, \vx'\in [0,1]^2}\|\vx-\vx'\|_1\Pr[\neg \mathcal{E}]\le 2\delta.$$
    The second term can be bounded by \Cref{lem:tvd2condi}.  Given $s_1\in \mathcal{S}_1$ and $s_2\in \mathcal{S}_2$, we set $\delta_1(s_1) = \sum_{w\in \Omega}|\Pr_\theta[w,s_1]-\Pr_{\theta'}[w,s_1]|$ and $\delta_2(s_2) = \sum_{w\in \Omega}|\Pr_\theta[w,s_2]-\Pr_{\theta'}[w,s_2]|$.  Then we have
    \begin{align*}
         &\E\left[\|\hat{\mathbf{X}}-\hat{\mathbf{X}}'\|_1\mid \mathcal{E}\right]\Pr[\mathcal{E}]\\
        =& \sum_{\vs}\Pr_\theta[\vs]\frac{\min(\Pr_\theta[\vs], \Pr_{\theta'}[\vs])}{\Pr_\theta[\vs]}\left\|\Pr_\theta[W|s_1]-\Pr_{\theta'}[W|s_1]\right\|_1+\left\|\Pr_\theta[W|s_2]-\Pr_{\theta'}[W|s_2]\right\|_1\\
         =& \sum_{\vs}\min(\Pr_\theta[\vs], \Pr_{\theta'}[\vs])\left\|\Pr_\theta[W|s_1]-\Pr_{\theta'}[W|s_1]\right\|_1+\sum_{\vs}\min(\Pr_\theta[\vs], \Pr_{\theta'}[\vs])\left\|\Pr_\theta[W|s_2]-\Pr_{\theta'}[W|s_2]\right\|_1\\
         \le& \sum_{s_1}\min(\Pr_\theta[s_1], \Pr_{\theta'}[s_1])\left\|\Pr_\theta[W|s_1]-\Pr_{\theta'}[W|s_1]\right\|_1+\sum_{s_2}\min(\Pr_\theta[s_2], \Pr_{\theta'}[s_2])\left\|\Pr_\theta[W|s_2]-\Pr_{\theta'}[W|s_2]\right\|_1\\
         \le& 2\sum_{s_1}\delta_1(s_1)+2\sum_{s_2}\delta_2(s_2)\tag{by \Cref{lem:tvd2condi}}\\
         \le& 4\delta\tag{$\sum_{s_1}\delta(s_1), \sum_{s_1}\delta(s_1)\le \delta$ }
    \end{align*}
    That completes the proof.
\end{proof}

Given a random variable $(W, S_1, S_2) \in \Omega\times \mathcal{S}_1\times \mathcal{S}_2$ with distribution $P$, if Alice only receives $S_1$ and Bob only receives $S_2$, we define Alice's \emph{second order forecast} as Alice's expectation for Bob's forecast given her signal $X_1^+\in \Delta_\Omega$ 
so that 
$$X_1^+ = \sum_{s_2} \Pr[W|S_2 = s_2]\Pr[S_2 = s_2|S_1 = s_1] = \E[\Pr[W|S_2]\mid s_1] \text{ with probability } \Pr[s_1].$$
Recall that we use $\Xdis{\theta}$ for prediction.  Similarly, we use $\Xdis{\theta}^+$ for the second order forecast.  The following result shows that the EMD of second order forecast under two information structures can be bounded by the TVD of signal distributions.
\begin{proposition}\label{prop:tv2second}
    Given two information structures $\theta$ and $\theta'$ on $\Omega\times \mathcal{S}_1\times\mathcal{S}_2$, 
    $$d_{EM}((\Xdis{\theta}, \Xdis{\theta}^+), (\Xdis{\theta'}, \Xdis{\theta'}^+))\le 16d_{TV}(\Sigdis{\theta}, \Sigdis{\theta'}).$$
\end{proposition}
\begin{proof}[proof for \Cref{prop:tv2second}]
Similar to \Cref{prop:tv2first}, we defined a coupling based on the maximal coupling on the signal space.  We first sample $(\hat{\vs}, \hat{\vs}')$ from the maximal coupling, and map the signals to $(\hat{\mathbf{X}}, \widehat{\mathbf{X}^+}) = (\Pr_\theta[W|[\hat{s_1}], \E_\theta[\Pr_\theta[W|S_2]\mid \hat{s_1}])$ and  
$(\hat{\mathbf{X}}', \widehat{\mathbf{X}^+}') = (\Pr_{\theta'}[W|\hat{s_1}'], \E_{\theta'}[\Pr_{\theta'}[W|S_2]\mid \hat{s_1}'])$.  Let $d_{TV}(\Sigdis{\theta}, \Sigdis{\theta'}) = \delta$.  Given above coupling, we can use triangle inequality and \Cref{prop:tv2first} to simplify the EMD bound,
\begin{equation}\label{eq:second1}
    d_{EM}((\hat{\mathbf{X}}, \widehat{\mathbf{X}^+}),(\hat{\mathbf{X}}', \widehat{\mathbf{X}^+}'))\le \E\left[\|\hat{\mathbf{X}}-\hat{\mathbf{X}}'\|_1\right]+\E\left[\|\widehat{\mathbf{X}^+}-\widehat{\mathbf{X}^+}'\|_1\right]\le 6\delta+\E\left[\|\widehat{\mathbf{X}^+}-\widehat{\mathbf{X}^+}'\|_1\right].
\end{equation}
Now we want to upper bound $\E\left[\|\widehat{\mathbf{X}^+}-\widehat{\mathbf{X}^+}'\|_1\right]$.  Using the identical argument as \Cref{prop:tv2first}, let $\mathcal{E}$ be the matching event, we have 
\begin{equation}\label{eq:second2}
    \E\left[\|\widehat{\mathbf{X}^+}-\widehat{\mathbf{X}^+}'\|_1\right]\le 2\delta+\E\left[\|\widehat{\mathbf{X}^+}-\widehat{\mathbf{X}^+}'\|_1\mid \mathcal{E}\right]\Pr[\mathcal{E}]
\end{equation}
Given $s_1\in \mathcal{S}_1$ and $s_2\in \mathcal{S}_2$, we set $\delta_1(s_1) = \sum_{w\in \Omega}|\Pr_\theta[w,s_1]-\Pr_{\theta'}[w,s_1]|$, $\delta_2(s_2) = \sum_{w\in \Omega}|\Pr_\theta[w,s_2]-\Pr_{\theta'}[w,s_2]|$, and $\delta_{1\to 2}(s_1) = \sum_{s_2'}|\Pr_\theta[s_1,s_2']-\Pr_{\theta'}[s_1,s_2']|$.  Note that by triangle inequality on \Cref{def:tvd}, the summation of all three terms are less than TVD
\begin{equation}\label{eq:tv2second1}
    \sum_{s_1} \delta_1(s_1), \sum_{s_2} \delta_2(s_2), \sum_{s_1} \delta_{1\to 2}(s_1)\le \delta
\end{equation}
By triangle inequality we have
\begin{align*}
    &\E\left[\|\widehat{{X_1}^+}-\widehat{{X_1}^+}'\|_1\mid \mathcal{E}\right]\Pr[\mathcal{E}]\\
    =& \sum_{\vs}\Pr_\theta[\vs]\frac{\min(\Pr_\theta[\vs], \Pr_{\theta'}[\vs])}{\Pr_\theta[\vs]}\left\|\E_\theta[\Pr_\theta[W|S_2]\mid s_1]-\E_{\theta'}[\Pr_{\theta'}[W|S_2]\mid s_1]\right\|_1\\
    \le& \sum_{s_1}\min(\Pr_\theta[s_1], \Pr_{\theta'}[s_1])\left\|\E_\theta[\Pr_\theta[W|S_2]\mid s_1]-\E_{\theta'}[\Pr_{\theta'}[W|S_2]\mid s_1]\right\|_1\\
    =& \sum_{s_1}\min(\Pr_\theta[s_1], \Pr_{\theta'}[s_1])\left\|\sum_{s_2}\Pr_\theta[s_2|s_1]\Pr_\theta[W|s_2]-\Pr_{\theta'}[s_2|s_1]\Pr_{\theta'}[W|s_2]\right\|_1\\
    \le& \sum_{s_1, s_2, w}\min(\Pr_\theta[s_1], \Pr_{\theta'}[s_1])\left|\Pr_\theta[s_2|s_1]\Pr_\theta[W|s_2]-\Pr_{\theta'}[s_2|s_1]\Pr_{\theta'}[W|s_2]\right|\\
    \le& \sum_{s_1, s_2, w}\min(\Pr_\theta[s_1], \Pr_{\theta'}[s_1])\left(\left|\Pr_\theta[s_2|s_1]\Pr_\theta[w|s_2]-\Pr_{\theta}[s_2|s_1]\Pr_{\theta'}[w|s_2]\right|+\left|\Pr_\theta[s_2|s_1]\Pr_{\theta'}[w|s_2]-\Pr_{\theta'}[s_2|s_1]\Pr_{\theta'}[w|s_2]\right|\right)\\
    =& \sum_{s_1, s_2, w}\min(\Pr_\theta[s_1], \Pr_{\theta'}[s_1])\Pr_\theta[s_2|s_1]\left|\Pr_\theta[w|s_2]-\Pr_{\theta'}[w|s_2]\right|+\sum_{s_1, s_2, w}\min(\Pr_\theta[s_1], \Pr_{\theta'}[s_1])\left|\Pr_\theta[s_2|s_1]-\Pr_{\theta'}[s_2|s_1]\right|\Pr_{\theta'}[w|s_2]
\end{align*}
For the first term, because $\sum_{s_1}\min(\Pr_\theta[s_1], \Pr_{\theta'}[s_1])\Pr_\theta[s_2|s_1] \le \sum_{s_1} \Pr_\theta[s_1, s_2] = \Pr_\theta[s_2]$, by \Cref{lem:tvd2condi}
\begin{align*}
    &\sum_{s_1, s_2, w}\min(\Pr_\theta[s_1], \Pr_{\theta'}[s_1])\Pr_\theta[s_2|s_1]\left|\Pr_\theta[w|s_2]-\Pr_{\theta'}[w|s_2]\right|\\
    \le& \sum_{s_2}\Pr_\theta[s_2]\sum_w\left|\Pr_\theta[w|s_2]-\Pr_{\theta'}[w|s_2]\right|\\
    \le& \sum_{s_2}\Pr_\theta[s_2]\frac{2}{\max \Pr_\theta[s_2], \Pr_{\theta'}[s_2]}\delta_2(s_2)\tag{by \Cref{lem:tvd2condi}}\\
    \le& 2\delta\tag{by \Cref{eq:tv2second1}}
\end{align*}
For the second term, because $\sum_w \Pr_{\theta'}[w|s_2] = 1$, 
\begin{align*}
    &\sum_{s_1, s_2, w}\min(\Pr_\theta[s_1], \Pr_{\theta'}[s_1])\left|\Pr_\theta[s_2|s_1]-\Pr_{\theta'}[s_2|s_1]\right|\Pr_{\theta'}[w|s_2]\\
    =& \sum_{s_1}\min(\Pr_\theta[s_1], \Pr_{\theta'}[s_1])\sum_{s_2}\left|\Pr_\theta[s_2|s_1]-\Pr_{\theta'}[s_2|s_1]\right|\\
    \le& \sum_{s_1}\min(\Pr_\theta[s_1], \Pr_{\theta'}[s_1])\frac{2}{\max \Pr_\theta[s_1], \Pr_{\theta'}[s_1]}\delta_{1\to 2}(s_1)\tag{by \Cref{lem:tvd2condi}}\\
    \le& 2\delta\tag{by \Cref{eq:tv2second1}}
\end{align*}
Therefore, $\E\left[\|\widehat{{X_1}^+}-\widehat{{X_1}^+}'\|_1\mid \mathcal{E}\right]\Pr[\mathcal{E}]\le 4\delta$ and $\E\left[\|\widehat{{X_2}^+}-\widehat{{X_2}^+}'\|_1\mid \mathcal{E}\right]\Pr[\mathcal{E}]\le 4\delta$ by symmetry.  Finally, by triangle inequality
$$\E\left[\|\widehat{\mathbf{X}^+}-\widehat{\mathbf{X}^+}'\|_1\mid \mathcal{E}\right]\Pr[\mathcal{E}]\le \E\left[\|\widehat{{X_1}^+}-\widehat{{X_1}^+}'\|_1\mid \mathcal{E}\right]\Pr[\mathcal{E}]+\E\left[\|\widehat{{X_2}^+}-\widehat{{X_2}^+}'\|_1\mid \mathcal{E}\right]\Pr[\mathcal{E}]\le 8\delta,$$
and by \Cref{eq:second1,eq:second2}
$$d_{EM}((\hat{\mathbf{X}}, \widehat{\mathbf{X}^+}),(\hat{\mathbf{X}}', \widehat{\mathbf{X}^+}'))\le 6\delta+2\delta+8\delta = 16\delta$$
which completes the proof.
\end{proof}

\begin{lemma}\label{lem:tvd2condi}
    Given two information structures $P$ and $Q$ on $\Omega\times \mathcal{A}$, for all $a\in \mathcal{A}$ the distance of prediction can be upper bounded,
    $$\|P[W|a]-Q[W|a]\|_1\le \frac{2}{\max(P[a],Q[a])}\sum_{w\in \Omega}|P[w,a]-Q[w,a]|.$$
\end{lemma}
\begin{proof}
    Given $a\in \mathcal{A}$, we set $\delta(a) = \sum_{w\in \Omega}|P[w,a]-Q[w,a]|$ and we have
    \begin{align*}
        \|P[W|a]-Q[W|a]\|_1=&\sum_{w\in \Omega}\left|P[w|a]-Q[w|a]\right|\\
        =& \frac{1}{P[a]Q[a]}\sum_{w\in \Omega}\left|P[w,a]Q[a]-Q[w,a]P[a]\right|\\
        =& \frac{1}{P[a]Q[a]}\sum_{w\in \Omega}\left|\sum_{w'\in \Omega}P[w,a]Q[w',a]-\sum_{w'\in \Omega}Q[w,a]P[w', a]\right|\\
        \le& \frac{1}{P[a]Q[a]}\sum_{w, w'\in \Omega}\left|P[w,a]Q[w',a]-Q[w,a]P[w', a]\right|\\
        \le& \frac{1}{P[a]Q[a]}\sum_{w, w'}\left|P[w,a]Q[w',a]-P[w,a]P[w',a]\right|+\left|P[w,a]P[w',a]-Q[w,a]P[w', a]\right|\\
        =& \frac{1}{P[a]Q[a]}\left(\sum_wP[w,a]\left(\sum_{w'}\left|Q[w',a]-P[w',a]\right|\right)+\left(\sum_{w'}P[w',a]\right)\sum_w\left|P[w,a]-Q[w,a]\right|\right)\\
        \le& \frac{1}{P[a]Q[a]}\left(P[a]\delta(a)+P[a]\delta(a)\right)\\
        =& \frac{2P[a]\delta(a)}{P[a]Q[a]}.
    \end{align*}
    Using similar argument, we have $\|P[W|a]-Q[W|a]\|_1\le \frac{2\delta(a)}{\max P[a], Q[a]}$ and complete the proof.
\end{proof}
\paragraph{Proof outline for second order case}
\begin{enumerate}
    \item As \Cref{lem:reduction}, show $\Thetabci$ is enough for the first order case.  We may use a similar argument to show $\Theta^{3ci} = \{\theta\in \Thetaci: |\mathcal{S}_i| = 3, \forall i\}$ is enough for the second order case.
    \item Construct a TV covering for signal space.  Here is a candidate: $\Theta^{3ci}_N = \{\theta\in \Theta^{3ci}: \mu, \Pr[s_i|w]\in [1/N], \forall s_i, w\}$ where the prior and conditional probability are multiples of $1/N$. 
    \item By \Cref{prop:tv2second}, we can show the above TV-covering for signal space is a EM-covering for first and second order predictions (similar to \Cref{l:smallcoverlipschitz}).   Then reuse \Cref{lem:dem_smooth}
    \item New algorithm for Liptchitz aggregator on first and second order prediction (simil\Cref{lem:lipbestresponsecomp} and \Cref{lem:liplosscomp}, \Cref{alg:2})
\end{enumerate}
\begin{proposition}
$\Theta^{?}_{N}$ is a good $TV$-coverings in signal space so that for all $\theta\in \Theta^{?ci}$, there exists $\theta'\in \Theta^{?}_{N}$ so that $d_{TV}((\mathbf{W}_\theta, \mathbf{S}_\theta), (\mathbf{W}_{\theta'}, \mathbf{S}_{\theta'}))\le \frac{1}{N}$
\end{proposition}
\begin{proposition}\label{prop:tv2em1}
    Given two information structures $P$ and $Q$ on $\Omega\times \mathcal{A}$,
    $$d_{EM}(X_P,X_Q)\le 4d_{TV}((W_P, A_P),(W_Q, A_Q))$$
    where $X_P$ is the distribution of posterior given an information structure $P$, $X_P = P[W|A = a]\in \Delta_\Omega$ with probability $P[a]$. 
\end{proposition}
\begin{proof}[Proof of \Cref{prop:tv2em1}]
Our coupling is derived from the maximal coupling between $P$ and $Q$ on the signal space.  Formally, we sample $a$ with probability $P[a]$ and output $\hat{X}_P = P[W|a]$.  Then, let $\hat{X}_Q = Q[W|a]$ with probability $\min(P[a], Q[a])/P[a]$ and any other feasible value that satisfies the marginal distribution so that $\hat{X}_P = X_P$ and $\hat{X}_Q = X_Q$ in distribution. 

Let $d_{TV}((W_P, A_P),(W_Q, A_Q)) = \delta$.  First we define the matching event as  
    $$\mathcal{E}:=\{(\hat{X}_P, \hat{X}_Q): \exists a\in \mathcal{A}, \hat{X}_P = P[W|a], \hat{X}_Q = Q[W|a]\}.$$  Then the probability of not matching is 
    \begin{equation}\label{eq:tv2em11}
        1-\sum_{a}P[a]\frac{\min(P[a], Q[a])}{P[a]} = \frac{1}{2}\sum_{a}|P[a]-Q[a]| = d_{TV}(A_P,A_Q)\le\delta
    \end{equation}
    The second equality is due to \Cref{def:tvd}.  By the duality form of EMD~\Cref{eq:dual}, we have
    $$d_{EM}(X_P,X_Q)\le \E\left[\|\hat{X}_P-\hat{X}_Q\|_1\right] = \E\left[\|\hat{X}_P-\hat{X}_Q\|_1\mid \neg \mathcal{E}\right]\Pr[\neg \mathcal{E}]+\E\left[\|\hat{X}_P-\hat{X}_Q\|_1\mid \mathcal{E}\right]\Pr[\mathcal{E}].$$
    We bound these two terms separately. First, because the one norm of the difference between two distributions is always bounded by $2$, by \Cref{eq:tv2first1}
    $$\E\left[\|\hat{X}_P-\hat{X}_Q\|_1\mid \neg \mathcal{E}\right]\Pr[\neg \mathcal{E}]\le 2\delta.$$
    For the second term, by \Cref{lem:tvd2condi} we have
    \begin{align*}
         &\E\left[\|\hat{X}_P-\hat{X}_Q\|_1\mid \mathcal{E}\right]\Pr[\mathcal{E}]\\
        =& \sum_{a}P[a]\frac{\min(P[a], Q[a])}{P[a]}\sum_w\left|P[w|a]-Q[w|a]\right|\\
        =& \sum_{a}\min(P[a], Q[a])\left(\frac{2\delta(a)}{\max P[a], Q[a]}\right)\tag{by \Cref{lem:tvd2condi}}\\
        \le& 2\sum_{a}\delta(a)\\
        =& 2\delta
    \end{align*}
    That completes the proof.
\end{proof}
Given a random variable $(W, A, B) \in \Omega\times \mathcal{A}\times \mathcal{B}$ with distribution $P$, if Alice only receives $A\in \mathcal{A}$ and Bob only receives $B\in \mathcal{B}$, we define Alice's \emph{second order forecast} as Alice's expectation for Bob's forecast given her signal $X_P^+\in \Delta_\Omega$ 
so that 
$$X_P^+ = \sum_{b} \Pr[W|B = b]\Pr[B = b|A = a] = \E[\Pr[W|B = b]\mid A = a] \text{ with probability } \Pr[ A = a].$$
The following result shows that the EMD of second order forecaset under two distributions $P$ and $Q$ can be bounded by the TVD of $P$ and $Q$.
\begin{proposition}\label{prop:tv2em2}
    Given two distributions $P$ and $Q$ on $\Omega\times \mathcal{A}\times \mathcal{B}$, 
$$d_{EM}(X_P^+, X_Q^+)\le 6d_{TV}((W_P,A_P,B_P), (W_Q,A_Q,B_Q)).$$
where $(W_P, A_P, B_P), (W_Q,A_Q,B_Q) \in \Omega\times \mathcal{A}\times \mathcal{B}$ is the random variable sampled from $P$ and $Q$ respectively
\end{proposition} 

\begin{proof}
For brevity, we use $P(a) = P[A = a]$, $P(b|a) = P[B = b|A = a]$, and $P(W|b) = P[W|B = b]\in \Delta_\Omega$.  Let $f_P(a) = \sum_b P(W|b)P(b|a)$ and $f_Q(a) = \sum_b Q(W|b)Q(b|a)$ for all $a\in \mathcal{A}$.  Then the second order forecasts satisfy $\Pr[X_P = f_P(a)] = P(a)$ and $\Pr[X_Q = f_Q(a)] = Q(a)$ for all $a$.  

Let $d_{TV}((W_P,A_P,B_P), (W_Q,A_Q,B_Q)) = \delta$, $\delta_A(a) = \sum_{w\in \Omega}|P[w,a]-Q[w,a]|$, $\delta_B(b) = \sum_{w\in \Omega}|P[w,b]-Q[w,b]|$, and $\delta_{A\to B}(a) = \sum_{b}|P[a,b]-Q[a,b]|$ for all $a$ and $b$.  Note that by triangle inequality on \Cref{def:tvd}, the summation of all three terms are less than TVD
\begin{equation}\label{eq:tv2em21}
    \sum_a \delta_A(a), \sum_b \delta_B(b), \sum_a \delta_{A\to B}(a)\le \delta
\end{equation}
To bound the EMD, we use the maximal coupling between $\hat{A}_P$ and $\hat{A}_Q$ as \Cref{prop:tv2em1} with the matching event $\mathcal{E}$, and have
$$d_{EM}(X_P^+, X_Q^+)\le 2\delta+\E[\|f_P(\hat{A}_P)-f_Q(a)\|_1\mid \mathcal{E}]\Pr[ \mathcal{E}].$$
By triangle inequalty, we have
\begin{align*}
    &\E[\|f_P(a)-f_Q(a)\|_1\mid \mathcal{E}]\Pr[ \mathcal{E}]\\
    =& \sum_a \min(P(a), Q(a))\cdot \sum_w \left|\sum_b P(w|b)P(b|a)-Q(w|b)Q(b|a)\right|\\
    \le& \sum_{w,a,b} \min(P(a), Q(a))\left|P(w|b)P(b|a)-Q(w|b)Q(b|a)\right|\\
    \le& \sum_{w,a,b} \min(P(a), Q(a))(|P(w|b)-Q(w|b)|P(b|a)+Q(w|b)|P(b|a)-Q(b|a)|)\\
    =& \sum_{w,a,b} \min(P(a), Q(a))|P(w|b)-Q(w|b)|P(b|a)+\sum_{w,a,b}\min(P(a), Q(a))Q(w|b)|P(b|a)-Q(b|a)|
\end{align*}
For the first term, because $\sum_a \min (P(a),Q(a))P(b|a) \le \sum_a P(a,b) = P(b)$,
$$ \sum_{w,a,b} \min(P(a), Q(a))|P(w|b)-Q(w|b)|P(b|a)\le \sum_{w,b} |P(w|b)-Q(w|b)|P(b)$$
Additionally, by \Cref{lem:tvd2condi}, $\sum_w|P(w|b)-Q(w|b)|\le \frac{2\delta_B(b)}{\max P(b), Q(b)}$ for all $b$.  Therefore, with \Cref{eq:tv2em21},
\begin{equation}\label{eq:tv2em22}
    \sum_{w,b} |P(w|b)-Q(w|b)|P(b)\le \sum_b \frac{2\delta_B(b)}{\max P(b), Q(b)}P(b) \le 2\delta.
\end{equation}

For the second term, because $\sum_w Q(w|b) = 1$, 
$$\sum_{w,a,b}\min(P(a), Q(a))Q(w|b)|P(b|a)-Q(b|a)|\le \sum_{a,b}\min(P(a), Q(a))|P(b|a)-Q(b|a)|.$$  Similarly, by \Cref{lem:tvd2condi} and \Cref{eq:tv2em21}, 
\begin{equation}
    \label{eq:tv2em23}\sum_{a,b}\min(P(a), Q(a))|P(b|a)-Q(b|a)|\le \sum_{a,b}\min(P(a), Q(a))\frac{2\delta_{A\to B}(a)}{\max P(a), Q(a)}\le 2\delta
\end{equation} 
By \Cref{eq:tv2em22,eq:tv2em23}, we have
$$\E[\|f_P(a)-f_Q(a)\|_1\mid \mathcal{E}]\Pr[ \mathcal{E}]\le 4\delta,$$
and complete the proof.
\end{proof}

\section{second order}
In the second order setting, in addition to the predictions $x_i=\Pr[\omega=1|s_i]$, each agent is asked to report their prediction for others reports. That is $p_i=\E[x_{1-i}|s_i]$. We assume the signals are i.i.d.. Suppose the information structures of two independent identical agents are $\Theta^{i}$.

\begin{lemma}[dimension reduction]
    Suppose $\Theta^{ti}=\{\theta\in\Theta^i:\forall i, |\mathcal{S}_i|=3\}$. Then for any aggregator $f$, $R(f,\Theta^i)=R(f,\Theta^{ti})$.
\end{lemma}

\paragraph{Coordinates} Since we only consider agents with 3 types of signals, we can use 5 parameters to represent an information structure:

\begin{equation}\label{eq:para2}
\begin{cases}
p_0=\Pr_{\theta}[s_i=0|\omega=1]\\
p_1=\Pr_{\theta}[s_i=1|\omega=1]\\
q_0=\Pr_{\theta}[s_i=1|\omega=0]\\
q_1=\Pr_{\theta}[s_i=1|\omega=0]\\
\mu=\Pr[\omega=1]
\end{cases}
.
\end{equation}

Again we can use another group of parameters:

\begin{equation}\label{eq:para1}
    \begin{cases}
f_1=\Pr_{\theta}[\omega=1|s_i=0]\\
f_2=\Pr_{\theta}[\omega=1|s_i=1]\\
f_3=\Pr_{\theta}[\omega=1|s_i=2]\\
o=\E_{x_i}[x_i|\omega=1]\\
z=\E_{x_i}[x_i|\omega=0]\\
\end{cases}.
\end{equation}

This lemma shows the bijection between these two coordinates:

\begin{equation}\label{eq:para1}
    \begin{cases}
p_0=\frac{f_1 (f_2 f_3 (-o+z+1)-f_2 z+z (o-f_3))}{z (f_1-f_2) (f_1-f_3)}\\
p_1=\frac{f_2 (f_1 (f_3 (o-z-1)+z)+z (f_3-o))}{z (f_1-f_2) (f_2-f_3)}\\
q_0=-\frac{(f_1-1) (f_2 (f_3 (o-z-1)+z)+z (f_3-o))}{(o-1) (f_1-f_2) (f_1-f_3)}\\
q_1=\frac{(f_2-1) (f_1 (f_3 (o-z-1)+z)+z (f_3-o))}{(o-1) (f_1-f_2) (f_2-f_3)}\\
\mu = \frac{z}{1 - o + z}\\
\end{cases}.
\end{equation}

\begin{proof}
    We have 
    \begin{equation}\label{eq:para1}
    \begin{cases}
f_1=\frac{\mu p_0}{\mu p_0+(1-\mu)q_0}\\
f_2=\frac{\mu p_1}{\mu p_1+(1-\mu)q_1}\\
f_3=\frac{\mu (1-p_0-p_1)}{\mu (1-p_0-p_1)+(1-\mu)(1-q_0-q_1)}\\
o=f_1p_0+f_2p_1+f_3(1-p_0-p_1)\\
\mu o+(1-\mu)z=\mu\\
\end{cases}.
\end{equation}
\end{proof}

The following lemma shows that

$$\Theta^{ti}_N=\{\theta\in\Theta^{ti}:f_0,f_1,f_2\in[1/N]\}$$

\begin{lemma}
    
\end{lemma}

\begin{lemma}[Small Covering]

$\Theta^{ti}_N$ is a $EMD$ covering of $\Theta^{ti}$

\end{lemma}

\begin{proof}
    By simple calculation we have 
    $$\Pr[x_1=f_1,x_2=f_1]=\mu p_0^2+(1-\mu)q_0^2=-\frac{\left(f_1^2 (o-1)-(f_1-1)^2 z\right) (z (f_2 (-f_3)+f_2+f_3-o)+f_2 f_3 (o-1))^2}{(o-1) z (f_1-f_2)^2 (f_1-f_3)^2 (o-z-1)}$$

    First we have $f_1\le z\le 1+z-o$ and $1-o\le 1-o+z$.

    \paragraph{Case 1: $f_2-f_1\ge \delta_N,f_3-f_2\ge \delta_N$}
    \begin{align*}
    |\frac{\partial \Pr[x_1=f_1,x_2=f_1]}{\partial f_1}|&=|\frac{2f_1\left(f_1^2-f_2 f_3\right)((-f_2f_3+f_2+f_3-o)z+f_2 f_3(o-1))^2}{z (f_1-f_2)^3 (f_1-f_3)^3 (o-z-1)}|\\
    &+|\frac{2(1-f_1)((f_1-2) f_1-f_2 f_3+f_2+f_3)(z (-f_2f_3+f_2+f_3-o)+f_2 f_3 (o-1))^2}{(o-1)(f_1-f_2)^3 (f_1-f_3)^3 (o-z-1)}|\\
    &\le \frac{2\left|f_1^2-f_2 f_3\right|\left(|-f_2f_3+f_2+f_3-o|+|f_2 f_3|\right)^2}{(f_1-f_2)^3 (f_1-f_3)^3}\\
    &+|\frac{2(1-f_1)((f_1-2) f_1-f_2 f_3+f_2+f_3)(z (1-o)+f_2 f_3 (1-o))^2}{(o-1)(f_1-f_2)^3 (f_1-f_3)^3 (o-z-1)}|\\
    &\le \frac{2\left|f_1^2-f_2 f_3\right|\left(|-f_2f_3+f_2+f_3-o|+|f_2 f_3|\right)^2}{(f_1-f_2)^3 (f_1-f_3)^3}\\
    &+|\frac{2(1-f_1)((f_1-2) f_1-f_2 f_3+f_2+f_3)(z+f_2 f_3)^2}{(f_1-f_2)^3 (f_1-f_3)^3}|\\
    &\le \frac{8}{\delta_N^6}+\frac{16}{\delta_N^6}\\
    &=\frac{24}{\delta_N^6}
    \end{align*}

    \begin{align*}
    |\frac{\partial \Pr[x_1=f_1,x_2=f_1]}{\partial f_2}|&=|\frac{2 \left(f_1^2 (o-1)-(f_1-1)^2 z\right) (z (f_1 (-f_3)+f_1+f_3-o)+f_1 f_3 (o-1))z (f_2 (f_3-1)-f_3+o)}{(o-1) z (f_1-f_2)^3 (f_1-f_3)^2 (o-z-1)}|\\
    &+|\frac{2 \left(f_1^2 (o-1)-(f_1-1)^2 z\right) (z (f_1 (-f_3)+f_1+f_3-o)+f_1 f_3 (o-1))f_2 f_3 (o-1)}{(o-1) z (f_1-f_2)^3 (f_1-f_3)^2 (o-z-1)}|\\
    &\le |\frac{2 \left(f_1^2 (o-1)-(f_1-1)^2 z\right) (z+f_1 f_3)}{(f_1-f_2)^3 (f_1-f_3)^2}|\\
    &+|\frac{2 \left(f_1(o-1)-(f_1-1)^2\right) (z+f_1 f_3)f_2f_3}{(f_1-f_2)^3 (f_1-f_3)^2}|\\
    &\le \frac{8}{\delta_N^5}+\frac{8}{\delta_N^5}\\
    &=\frac{16}{\delta_N^5}
    \end{align*}

    By symmetry, 
    $$|\frac{\partial \Pr[x_1=f_1,x_2=f_1]}{\partial f_3}|\le \frac{16}{\delta_N^5}.$$

    \begin{align*}
    |\frac{\partial \Pr[x_1=f_1,x_2=f_1]}{\partial o}|&=|\frac{2 z (f_2+f_3-z-1) (f_2 (f_3 (o-z-1)+z)+z (f_3-o))}{(f_1-f_2)^2 (f_1-f_3)^2 (o-z-1)^3}|\\
    &\le |\frac{2 (f_2+f_3-z-1) (f_2(o(o-z-1)+z)+z(1-o))}{(f_1-f_2)^2 (f_1-f_3)^2 (1+z-o)^2}|\\
    &\le |\frac{2 (f_2+f_3-z-1)2(f_2+1) }{(f_1-f_2)^2 (f_1-f_3)^2}|\\
    &\le \frac{8}{\delta_N^4}
    \end{align*}

    \paragraph{Case 2:$f_2-f_1\le \delta_N,f_3-f_2\le \delta_N$}
    Then the mover takes at most $2\delta_N$.

    \paragraph{Case 3:$f_2-f_1\le \delta_N,f_3-f_2\ge \delta_N$}
    We have $|\Pr[x_1=f_3,x_2=f_3]-\Pr[x_1=f_3',x_2=f_3']|\le \nabla\Pr[x_1=f_3'',x_2=f_3'']\le \frac{18}{\delta_N^6}$.

    We want to show $\Pr[x_1=f_1,x_2=f_1]+\Pr[x_1=f_2,x_2=f_2]$

    \paragraph{Case 4:$f_2-f_1\ge \delta_N,f_3-f_2\le \delta_N$}
    The same.
    
\end{proof}

\begin{lemma}
    
\end{lemma}
